# Supplementary material for: PLATO: Pointer Learner for Agent and Task Openness
Source: arXiv:2607.25082 source file (2026-07-29)
Supplement: Supplementary file 1 [file Technical_Appendix.tex]

% tech_appendix.tex
\documentclass[letterpaper,oneside]{article}
\usepackage[letterpaper,left=1in,right=1in,top=1in,bottom=1in]{geometry}

% Use the SAME IJCAI style package you use in main.tex.
% Example (replace with your actual one):
%\usepackage{ijcai26}

\usepackage{times}
\usepackage{helvet}
\usepackage{courier}
\usepackage{graphicx}
\usepackage{booktabs}
\usepackage{amsmath,amssymb}
\usepackage{chngcntr}
\usepackage[hidelinks]{hyperref}
\usepackage{amsthm}

\title{Technical Appendix (Supplementary)}
% Keep authors EMPTY for anonymized submission
\author{}
\date{}          
\begin{document}
\maketitle

% ==========================
% Appendix numbering
% Appendix sections: A, B, ...
% Figures/Tables: A.1, A.2, ...
% ==========================
% ===== Appendix section numbering (A, B, ...)
\appendix
\renewcommand{\thesection}{A}
\renewcommand{\thesubsection}{A.\arabic{subsection}}
\renewcommand{\thesubsubsection}{A.\arabic{subsection}.\arabic{subsubsection}}

%\section{Appendix}\label{sec:appendix}
\input{sections/12-appendix}
\clearpage

\bibliographystyle{named}
\bibliography{references}

\end{document}
